# Supplementary material for: Deep learning meets nanophotonics: A generalized accurate predictor for near fields and far fields of arbitrary 3D nanostructures
Source: arXiv:1909.12056 ancillary file (2019-11-13)
Supplement: Supplementary file 1 [file supporting_information.pdf]

# Supporting informations for: Deep learning meets nanophotonics: A generalized accurate predictor for near fields and far fields of arbitrary 3D nanostructures

Peter R. Wiecha[1,*] and Otto L. Muskens[1,†]

[1] *Physics and Astronomy, Faculty of Engineering and Physical Sciences, University of Southampton, Southampton, UK*

## I. COUPLED DIPOLES: GREEN DYADIC METHOD

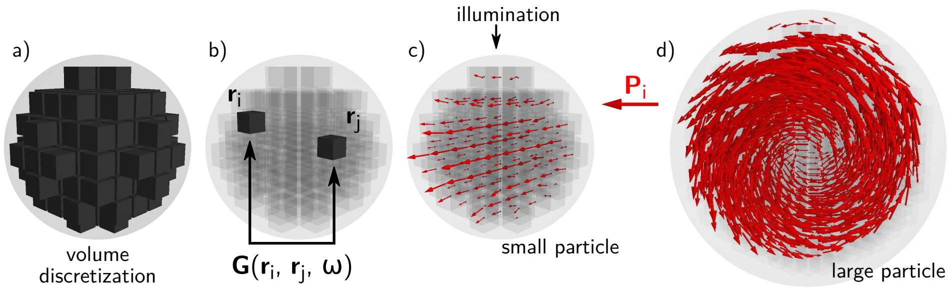


FIG. S1. Coupled dipole approximation at the example of a dielectric sphere. (a) Volume discretization of the nanoparticle. (b) Dipolar polarizabilities are assumed for each cell of the discretization. The self-consistent fields are calculated through evaluation of the coupling between all pairs of cells. (c-d) Illustration of the self-consistent electric polarization distribution $\mathbf{P}(\mathbf{r})$ inside the particle for a small (c) and large (d) silicon sphere.

The field at every meshcell inside the nanostructure can be calculated for instance using the Green Dyadic Method (GDM).[S1] In the GDM, the nanostructure is discretized in cubic elements of side-length $d$ (figure S1a) and each of these mesh-points is treated as an oscillating electric dipole with an effective, isotropic polarizability (cgs units)

$$\alpha(\mathbf{r}_i, \omega) = \frac{\epsilon_i(\omega) - \epsilon_{\text{env}}(\omega)}{4\pi} \cdot V_{\text{cell}} \,. \tag{S1}$$

The permittivity $\epsilon_i$ corresponds to the material of the nanostructure at location $\mathbf{r}_i$. $\epsilon_{\text{env}}$ is the isotropic and homogeneous permittivity of the environment.

From the optical wave-equation, a relation between the incident field and the field inside the nanostructure can be derived, leading ultimately to a set of $3N$ coupled linear equations (with $N$ the number of meshpoints):[S2]

$$\mathbf{E}_0 = \mathbf{M} \cdot \mathbf{E} \tag{S2}$$

where the matrix $\mathbf{M}$ consists of $3 \times 3$ sub-matrices

$$\mathbf{M}_{ij} = \mathbf{I} \cdot \delta_{ij} - \alpha(\mathbf{r}_i, \omega)\, \mathbf{G}_{\text{env}}(\mathbf{r}_i, \mathbf{r}_j, \omega) \,. \tag{S3}$$

Here, $\mathbf{I}$ is the Cartesian unitary tensor, $\delta_{ij}$ the Kronecker delta function and $\mathbf{G}_{\text{env}}$ is the Green's Dyad for the environment, coupling the dipolar elements $i$ and $j$ (see Fig. S1b). Additionally to the vacuum-tensor $\mathbf{G}_0$, further Dyads can be added to the Green's tensor, like a surface term $\mathbf{G}_{\text{s}}$ to account for the influence of a substrate:[S3]

$$\mathbf{G}_{\text{env}}(\mathbf{r}_i, \mathbf{r}_j, \omega) = \mathbf{G}_0(\mathbf{r}_i, \mathbf{r}_j, \omega) + \mathbf{G}_{\text{s}}(\mathbf{r}_i, \mathbf{r}_j, \omega) \,. \tag{S4}$$

Finally, to handle the divergence of the vacuum Green's function at $\mathbf{r}_i = \mathbf{r}_j$, a normalization scheme is applied:

$$\mathbf{G}_0(\mathbf{r}_i, \mathbf{r}_i, \omega) = \mathbf{I}\, C(\omega) \tag{S5}$$

---

* e-mail : p.wiecha@soton.ac.uk
† e-mail : o.muskens@soton.ac.uk

which, for a cubic discretization grid, gives[S4]

$$C(\omega) = -\frac{4\pi}{3}\frac{1}{\epsilon_{\text{env.}}(\omega) v_{\text{cell}}} \,. \tag{S6}$$

Inversion of the matrix $\mathbf{M}$ then directly leads to the electric field inside the structure $\mathbf{E}(\omega)$ upon excitation by an arbitrary illumination field $\mathbf{E}_0(\omega)$. The polarization of every cell – assuming linear, isotropic materials – is finally given by $\mathbf{p}(\mathbf{r}_i, \omega) = \chi_i(\omega)\mathbf{E}(\mathbf{r}_i, \omega)$ with $\chi_i(\omega) = (\epsilon_i(\omega) - \epsilon_{\text{env}}(\omega))/4\pi$, where $\mathbf{p}$ effectively represents an electric dipole moment.

The assumption that the meshpoints of the discretized particle can be described by dipolar polarizabilities allows us now to treat every discretization cell of the structure as an oscillating dipolar source of radiation. In this approximation, once the dipole moments $\mathbf{p}(\mathbf{r}_i, \omega)$ at all mesh positions $\mathbf{r}_i$ are known (Fig. S1c-d), the scattered field at any location $\mathbf{r}$ outside the structure can be calculated as the coherent sum of the fields emitted by the ensemble of dipoles:

$$\mathbf{E}_{\text{scat}}(\mathbf{r}, \omega) = \sum_{i=0}^{N} \mathbf{G}_{\text{env}}(\mathbf{r}, \mathbf{r}_i, \omega) \cdot \mathbf{p}(\mathbf{r}_i, \omega) \,. \tag{S7}$$

$\mathbf{G}_{\text{env}}$ is the Green's dyad for the environment without the nanostructure. Using the according mixed electric-magnetic Green's Dyad, also the optical magnetic field (and in consequence also the Poynting vector) can be obtained in both, the near- and the far-field region.[S1,S2]

## II. GEOMETRIC MODELS

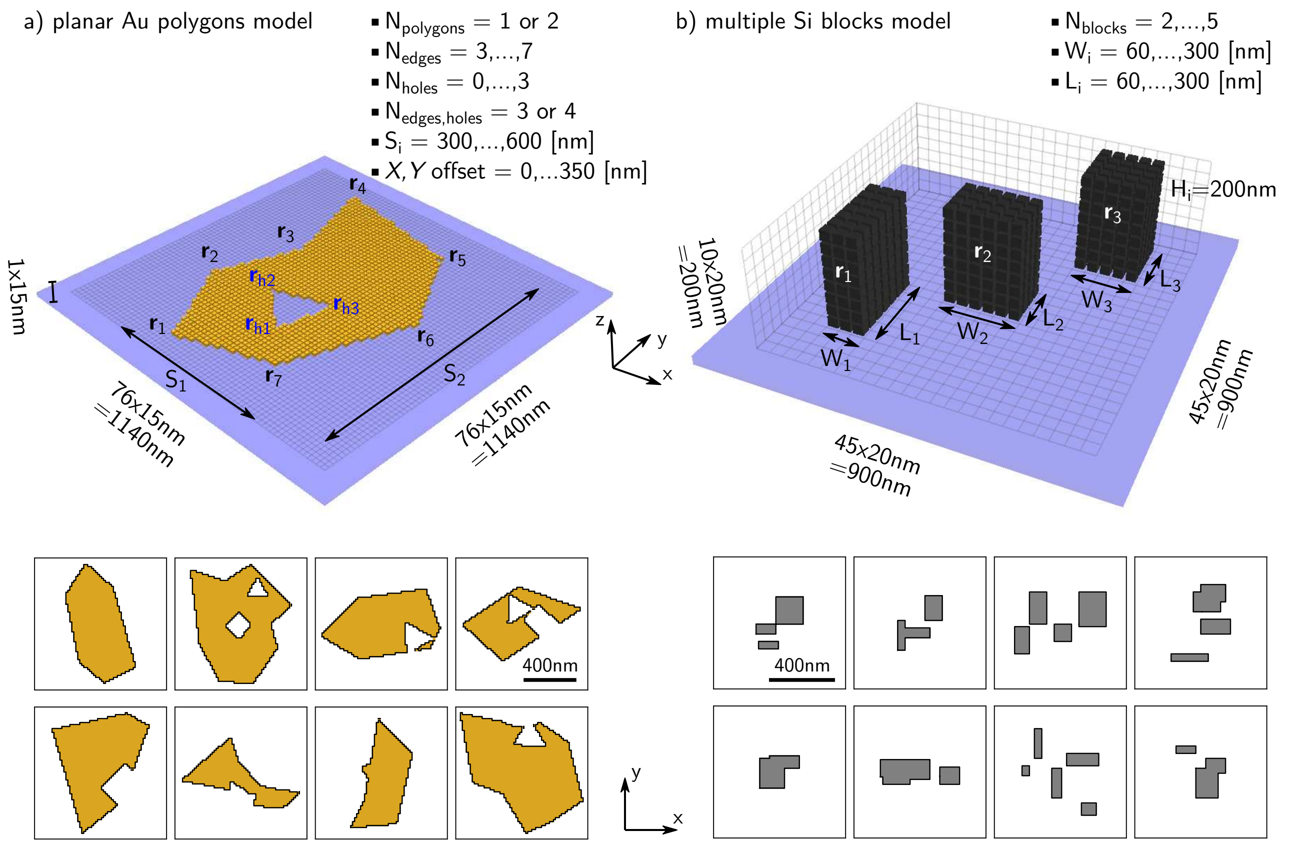


FIG. S2. Artistic sketches of the geometric models used (a) for the planar gold structures and (b) for the silicon nanostructures. While the top illustrations are not on absolute scales, several random examples of the actual training data are shown below.

Figure S2(a) shows the geometric model and parameter ranges used for generating the training data of the planar gold nanostructure internal field predictor network. We use a polygonal structure with up to 10 random edges $\mathbf{r}_i$, oriented along an elliptical shape with two random major axis lengths $S_1$ and $S_2$. The edge coordinates are uniformly distributed on the ellipse and then randomly shifted by up to half the major axis length in both directions. In case two polygons are generated, they are additionally moved by random $X$ and $Y$ offsets. Overlapping parts are fused together. In a second step, a random number of smaller polygonal holes are introduced, where we proceed in the same way as for the large polygon. The structures are finally randomly rotated on the $XY$ plane. The structures are discretized on a grid with stepsize 15 nm. Occasionally occurring structures which cover a larger area than the ANN input layer of $76 \times 76$ cells, are discarded. Gold refractive index is taken from Ref. S5.

The Si structures consist of a random number of cuboidal blocks of random lateral dimensions. For convenience, the height is set constant to 200 nm, but we emphasize that thanks to the fully 3D convolutional neural network architecture, this is not a requirement of the approach. The blocks are discretized with a stepsize of 20 nm and are randomly placed in an area of $45 \times 45$ steps. Overlapping blocks are fused together. Silicon refractive index taken from Ref. S6.

The geometries are fed into the input layer of the according gold or silicon ANN. If a position in the 3D grid is occupied by material, the according element in the input layer is set to “1”. If there is no gold (respectively silicon), it is set “0”.

## III. IMPLEMENTATION DETAILS OF THE 3D FULLY CONVOLUTIONAL NEURAL NETWORK

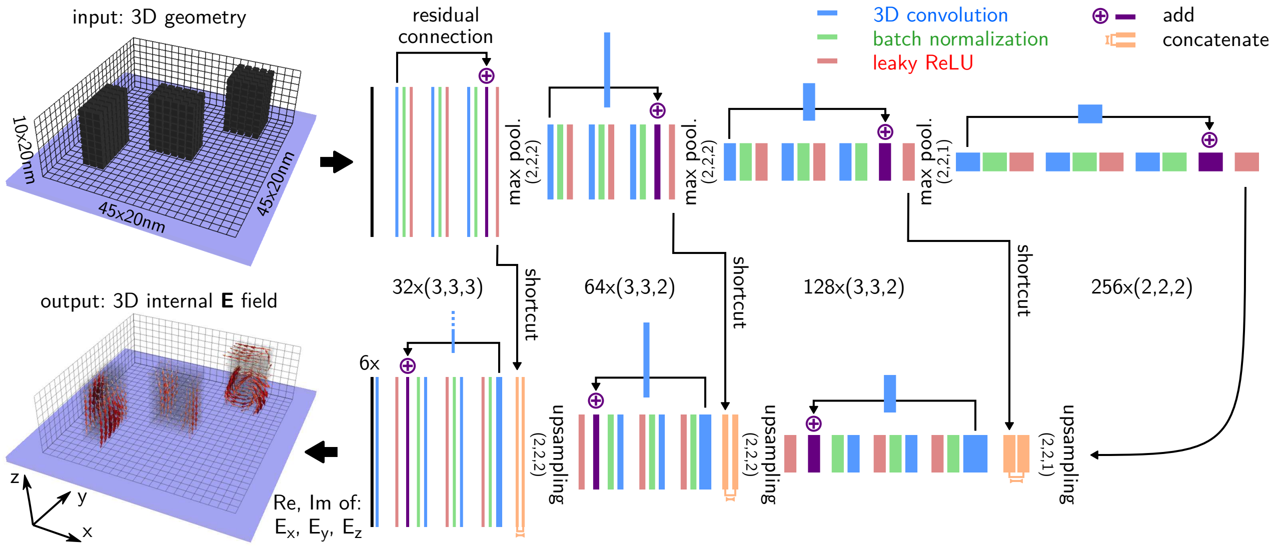


FIG. S3. Sketch of the 3D convolutional artificial neural network layout at the example of the silicon predictor network. The three-dimensional geometry (illustration on top left) is fed into the input layer of the ANN as an array of size ($45 \times 45 \times 10$), containing a value 0 (no silicon) or 1 (silicon) for every cell point of the discretized volume. The fully convolutional network follows an encoder-decoder architecture and is organized in a sequence of residual blocks, each of which containing three successive convolutional operations followed by batch normalization and a leaky rectifying linear unit nonlinearity ("leaky ReLU" with $\alpha = 0.1$). Residual connections including each a further convolutional layer are used to allow the learning to form identity operations which helps for efficient back-propagation of gradients and accelerates training of deep ANNs.[S7] Additionally we implement shortcut connections between the last leaky ReLU of the encoder stage blocks which we concatenate to the input layers of the residual blocks in the decoder part. This has been demonstrated to significantly improve reconstruction of fine spatial features.[S8] Finally, the network returns six output layers with linear activation, each having the same dimensions as the network input layer. Those six layers which contain the real and imaginary parts of the $x$, $y$ and $z$ components of the complex electric field inside the nanostructure (see illustration on bottom left). 3D convolutional kernel dimensions are indicated in parentheses.

We use a three-dimensional fully convolutional neural network for the prediction of the internal electric polarization of the nanostructures, as illustrated in figure S3. We construct a symmetric, fully convolutional network with "U-Net"[S8] type shortcut connections between corresponding convolutional and up-sampling units. These shortcut connections between the down- and up-sampling blocks (top, respectively bottom part in the network illustration in Fig. S3) help to accurately reconstruct spatial information from the strongly compressed center layers of the ANN. To be able to efficiently train the very deep networks, we organize the network in residual blocks[S7,S9]. The layer dimensions of the residual blocks in the down-sampling part of the ANN are successively reduced using "max pooling" operations, the number of kernels is doubled after each pooling layer. In the decoder part of the ANN (bottom in Fig. S3), we reconstruct spatial information from the compressed layers using residual blocks and "up-sampling" layers, arranged in a symmetric configuration with respect to the down-sampling part of the network. To preserve the dimensions used in the encoder stage, "zero padding" is applied following the up-sampling operations, if necessary.

In the case of the planar gold nanostructures, the $Z$ dimension of the geometry consists of a single layer of mesh points. So the third dimension of all layers and kernel filters is set equal 1 in this case.

Training was done for both datasets on mean square error loss using the ADAM optimizer at a learning rate of 0.00005 and with a batch size of 64.

## IV. NEAR- AND FAR-FIELD PREDICTION EXAMPLES FROM THE VALIDATION DATA

In figure S4 and figure S5, we show validation set examples for the gold, respectively silicon networks and compare derived physical observables to numerical simulations. The figures show examples with decreasing prediction performance from top (i) to bottom (vi). The last two rows in both figures represent "outliers" in terms of the boxplots in the main text figure 5.

Figures S4 and S5 (a) show near-field intensity maps in the vicinity of the nanostructure. (b) shows back focal plane (BFP) backscattering intensity plots. (c) shows scattering radiation pattern in the $XZ$ plane. (d) shows the far field polarization state of backscattered light.

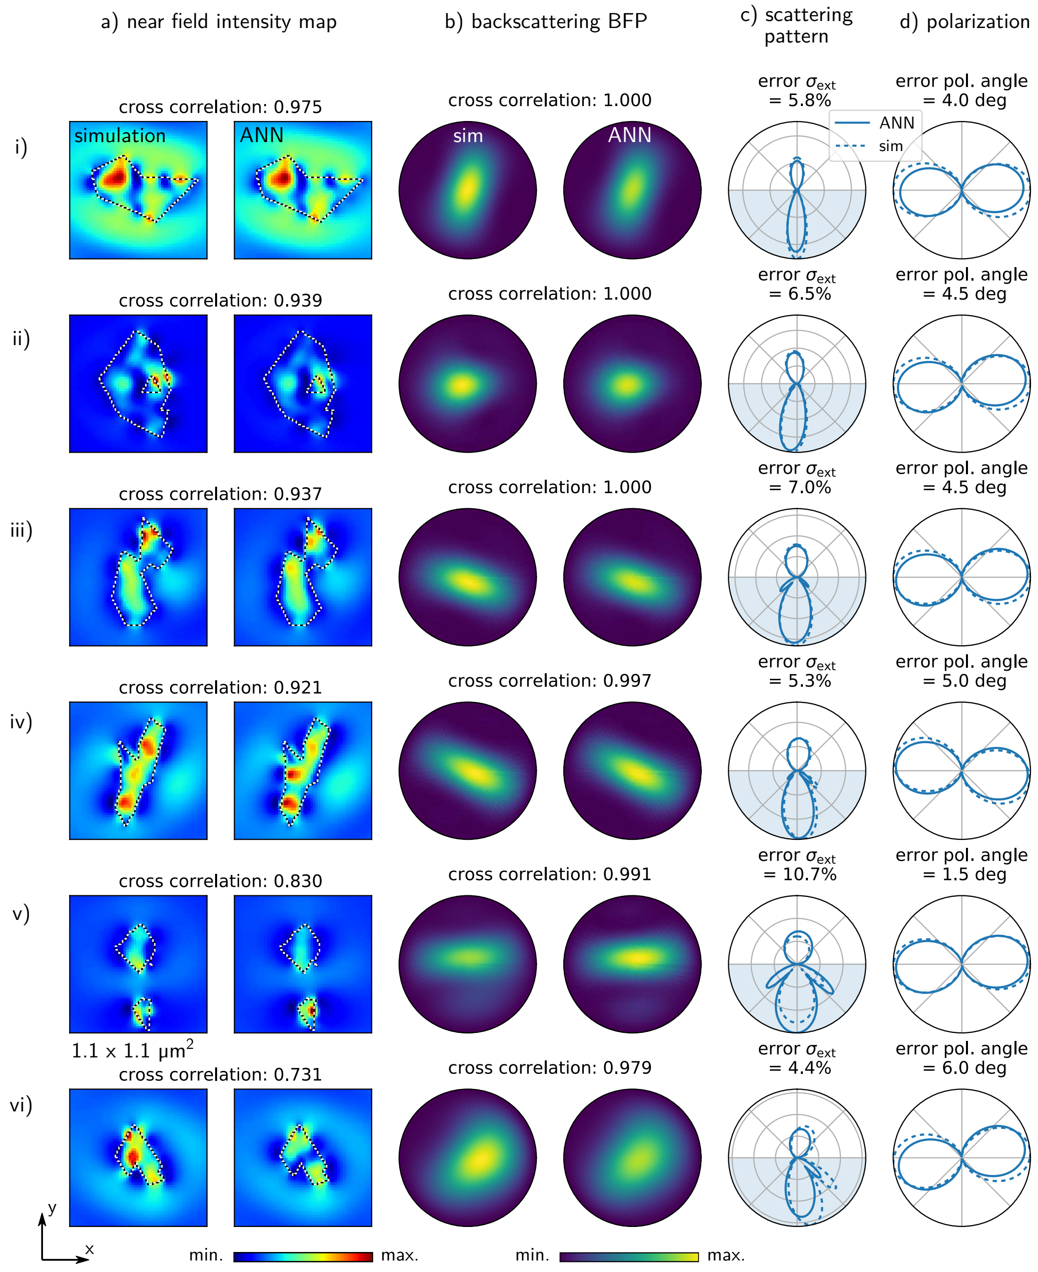


FIG. S4. Representative gold nanostructures from the validation set. Examples were chosen that show decreasing prediction fidelity from top (i) to bottom (vi). (a) near-field intensity 30 nm above the nanostructure. Shown areas are $1.1 \times 1.1\,\mu$m. (b) back focal plane image. (c) far-field scattering pattern in $XZ$ plane. (d) far-field backscattering polarization state.

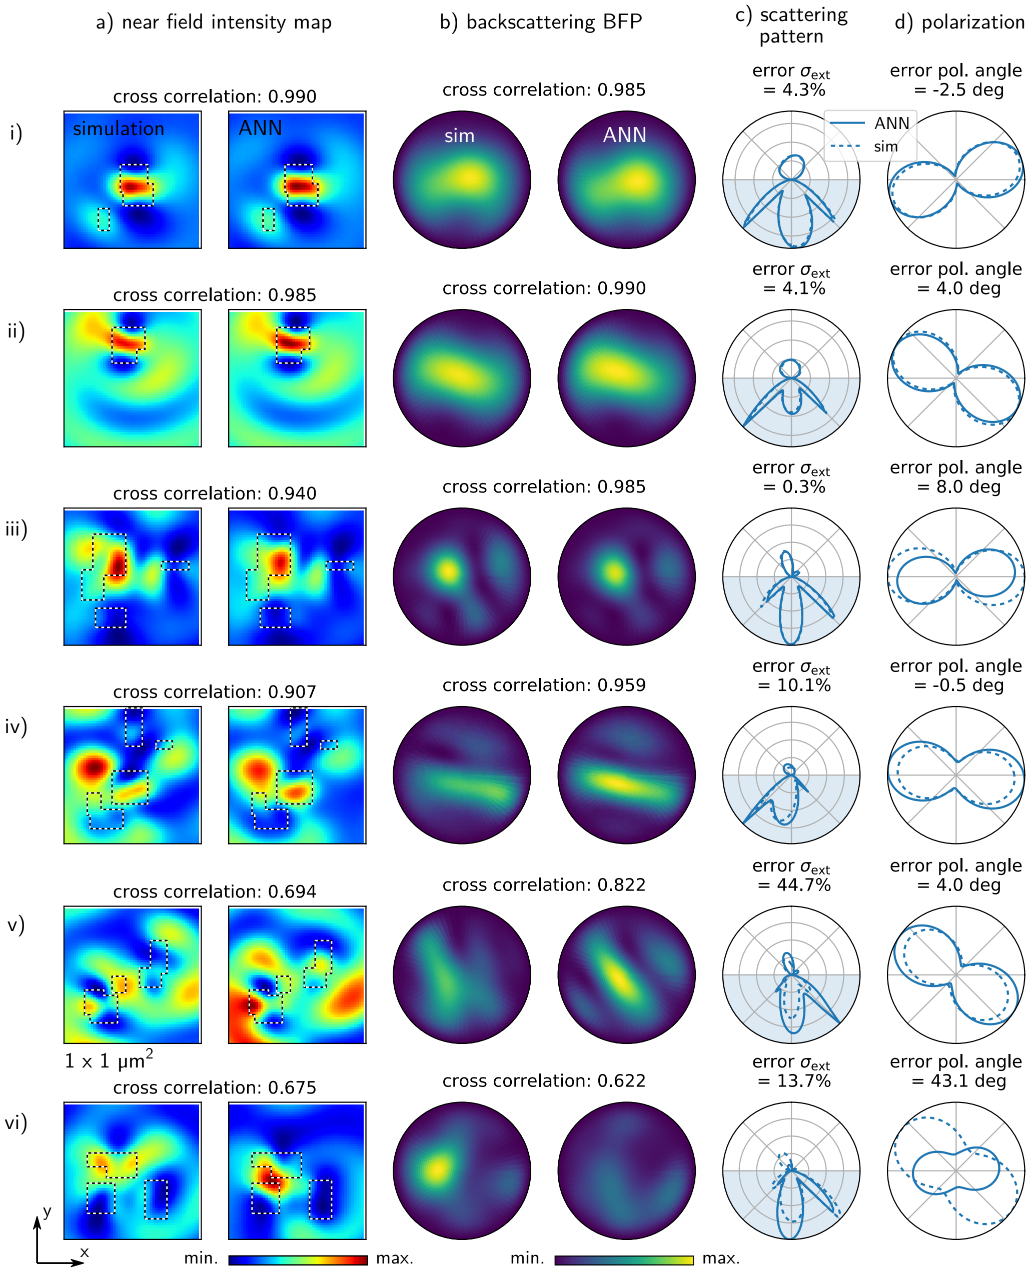


FIG. S5. Representative silicon nanostructures from the validation set. Examples were chosen that show decreasing prediction fidelity from top (i) to bottom (vi). (a) near-field intensity in the glass substrate, 100 nm below the nanostructure. Shown areas are $1 \times 1\,\mu m$. (b) back focal plane image. (c) far-field scattering pattern in $XZ$ plane. (d) far-field backscattering polarization state.

## V. GOLD NANO-DIMER: NEAR-FIELD INTERACTIONS; OPTICAL CHIRALITY

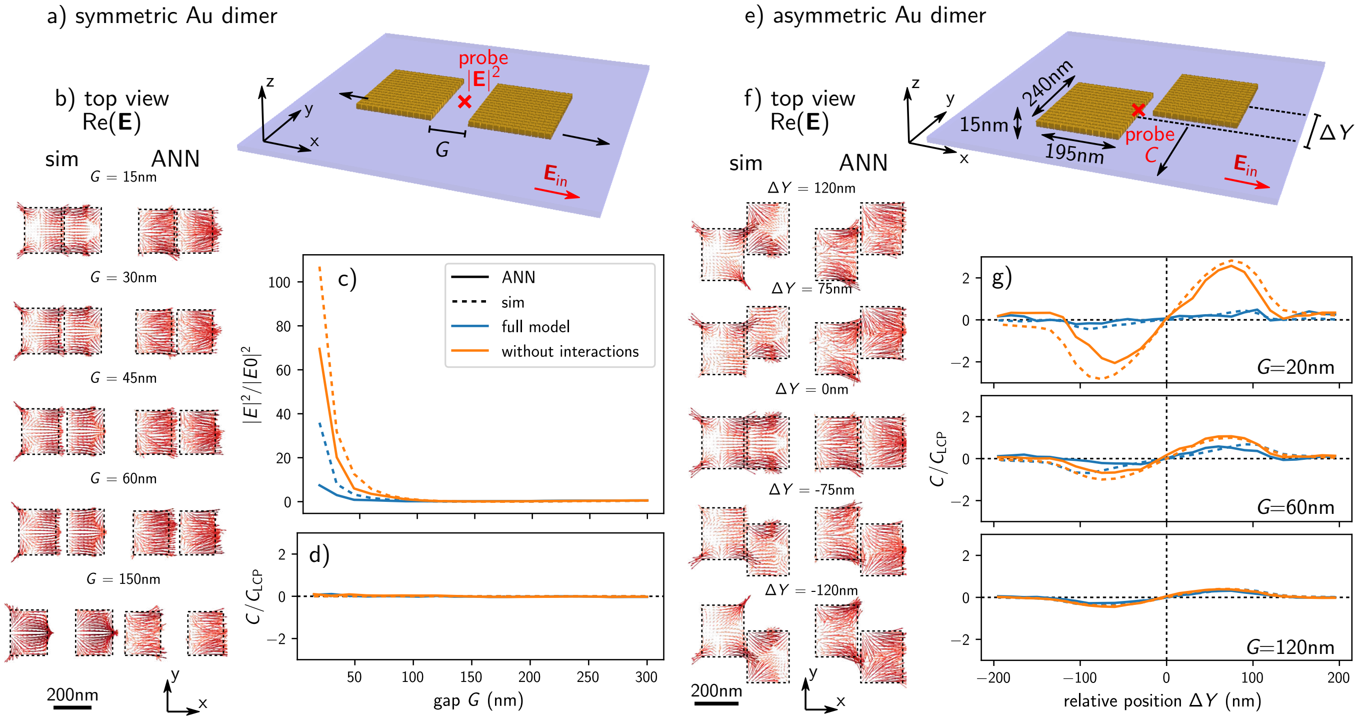


FIG. S6. Reproducibility of near-field enhancement and optical chirality at the example of a gold dimer. (a) Sketch of the symmetric gold dimer (each pad $195 \times 240 \times 15\,\text{nm}^3$). (b) Top view of the electric field vectors inside the gold pads upon $X$ polarized plane wave illumination, incident from the top for different gaps sizes. Left column: numerical simulation, right column: ANN prediction. (c) Field enhancement in the center of the gap (red cross in (a)), calculated from the ANN prediction (solid lines) or with numerical simulations (dashed lines). (d) optical chirality $C$ at 30 nm above the gap center (red cross in (e)), normalized to the chirality $C_{\text{LCP}}$ of a left-circular polarized plane wave. (e) Sketch of asymmetric gold dimer. One constituent is vertically shifted by a distance $\Delta Y$ relative to the other. (f) Same as (b) for the asymmetric dimer and different relative positions $\Delta Y$. (g) optical chirality $C$, normalized to $C_{\text{LCP}}$, calculated 30 nm above the middle of the gap, vertically centered at the left gold pad (red cross in (e)). Full field simulations (blue lines) are compared to calculations in which optical interactions have been artificially turned off (orange lines), see main text. All data were taken for a normally incident plane wave ($\mathbf{k}$ along $-Z$, $\lambda_0 = 700\,\text{nm}$), with linear polarization along $OX$.

To assess the ability of the neural network to predict near-field interactions between two particles, we show in the main text a nano-dimer built from two silicon blocks. Here we show the plasmonic counterpart made from a single layer of 15 nm high gold mesh cells, predicted by the planar gold polygon network.

As in the case of silicon dimers, the general trends are predicted by the neural network, yet with less accuracy in the gold case. We attribute this mainly to the fact that the gold dimer structure is entirely different than what the polygonal structures, the network was trained on. Most importantly, the training dataset contains almost no structures with gaps, whereas very particular effects occur due to strong coupling in plasmonic structures with small gaps. This is the reason why the near-field enhancement at very short distances is incorrectly predicted (figure S6c). This conclusion is further supported by the case of deactivated near-field interactions (orange lines S6c), where the network prediction agrees much better to the simulations, than in the case with interactions. Despite the rather limited capability of extrapolation to scenarios including strong optical near-field interactions, the general qualitative trend is correctly predicted also by the ANN, as the coupling between the two pads at short distances reduces significantly the electric field intensity in the gap in the here shown case.

The same conclusions hold also for the asymmetric dimer, shown in figure S6(e-g). While in the near-field quiver plots (Fig. S6f) again the limited accuracy of the predictions become visible under conditions of small gap coupling, the general trends for the optical chirality as here chosen near-field observable are consistent with simulations. The study also reveals an interesting behavior in the gold case. While in silicon dimers, coupling between the two blocks is the reason which gives rise to a significant near-field chirality, in case of the gold dimer optical interactions between the two pads quench the near-field chirality above the gap.

## VI. ARBITRARY ILLUMINATION POLARIZATION STATES

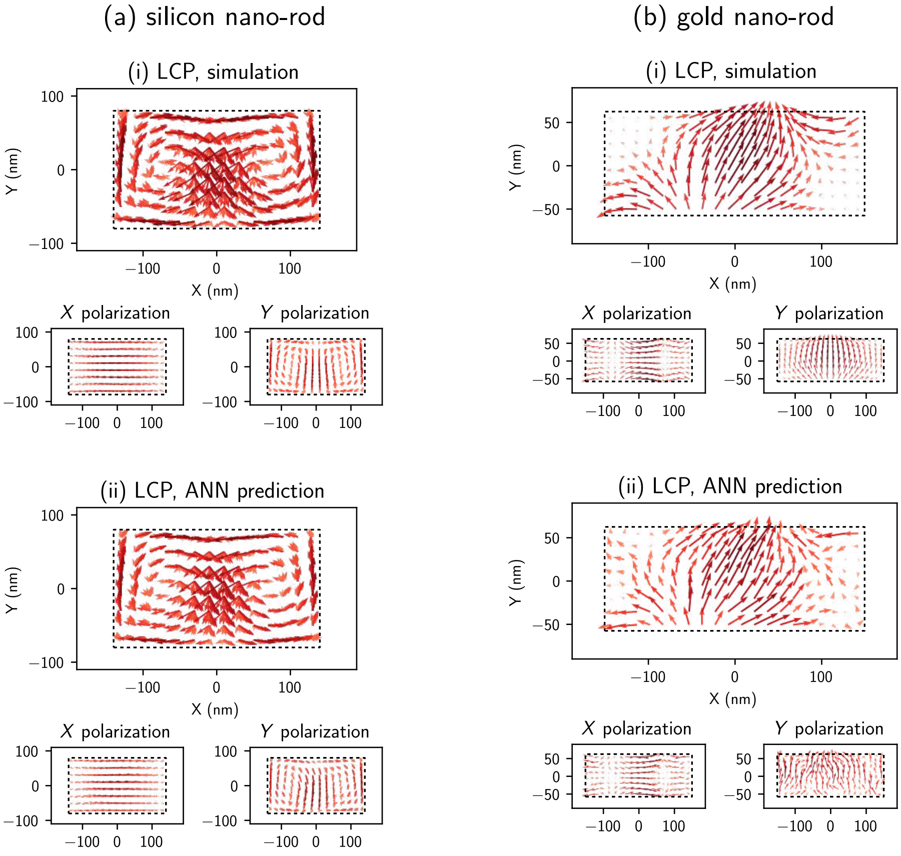


FIG. S7. Top view of simulated (i) and predicted (ii) internal field vectors (real part) under left circular polarized plane wave excitation for (a) silicon nano-rod and (b) planar gold nano-rod. Calculated from superposition of linear polarization. Below the LCP vector-plots, the according $X$- and $Y$-polarization cases are shown in small panels. $\lambda_0 = 700\,\text{nm}$.

Since we calculate and predict the linear response to fully coherent incident fields, it is possible to calculate the optical response to arbitrary polarization states of the illuminating plane wave through a superposition of two incident plane waves with perpendicular linear polarization. In consequence, our network can also be used to predict any elliptical incident polarization. For example, the internal field of a nanostructure upon illumination with left circular polarization (LCP) is identical to a superposition of the internal fields under $X$ polarized and under $Y$ polarized plane wave illumination, with an additional phase of $\pi/2$ for the $Y$-polarized response. Using complex fields, the LCP response is hence:

$$\mathbf{E}_{\text{LCP}} = \sqrt{\frac{1}{2}}\,\mathbf{E}_{\text{linear},X} + \mathrm{i}\,\sqrt{\frac{1}{2}}\,\mathbf{E}_{\text{linear},Y} \tag{S8}$$

To illustrate this, the internal fields for LCP plane wave illumination in a rectangular gold pad as well as in a silicon nano-rod are shown in figure S7. Simulated fields and ANN prediction are in very good agreement.

## VII. PERFORMANCE ON CURVED STRUCTURES

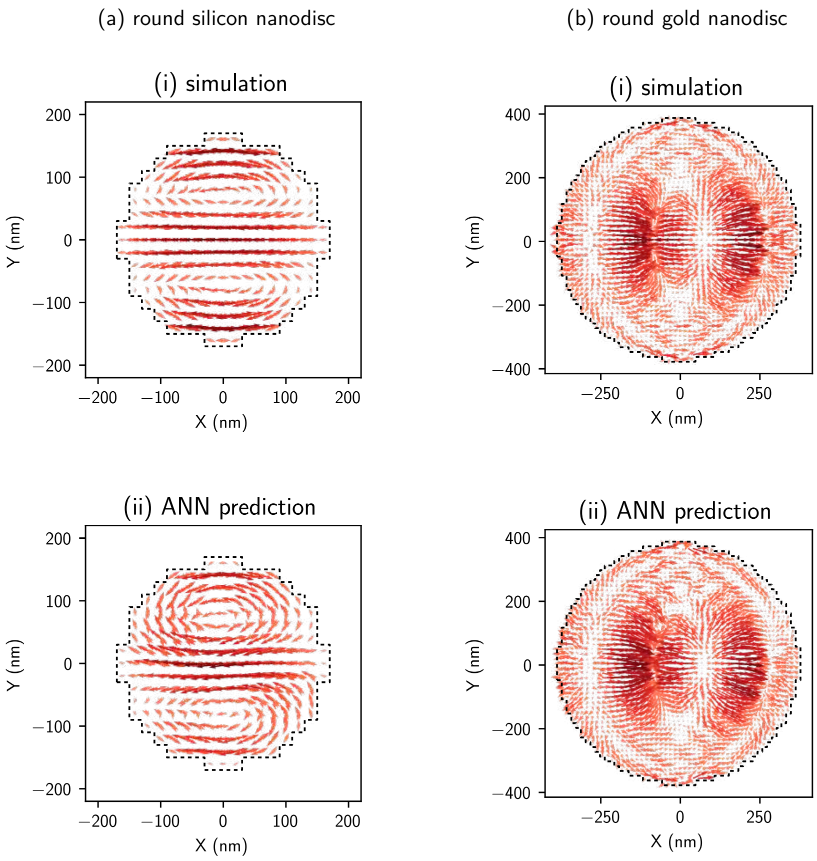


FIG. S8. Top view of simulated (i) and predicted (ii) internal field vectors (real part) under $X$ polarized plane wave illumination of (a) a silicon nano-disc and (b) a planar gold nano-disc. $\lambda_0 = 700\,\mathrm{nm}$.

Both networks in our demonstration use training data based on polygonal geometric models with flat facets (planar polygons for the gold network, multiple cuboids for the silicon network). In order to roughly estimate how well the networks manage to generalize to curved structures, we compare simulations of gold and silicon nano-discs to the respective network predictions.

## VIII. PREDICTION PERFORMANCE ON VARIABLE HEIGHT SILICON STRUCTURES

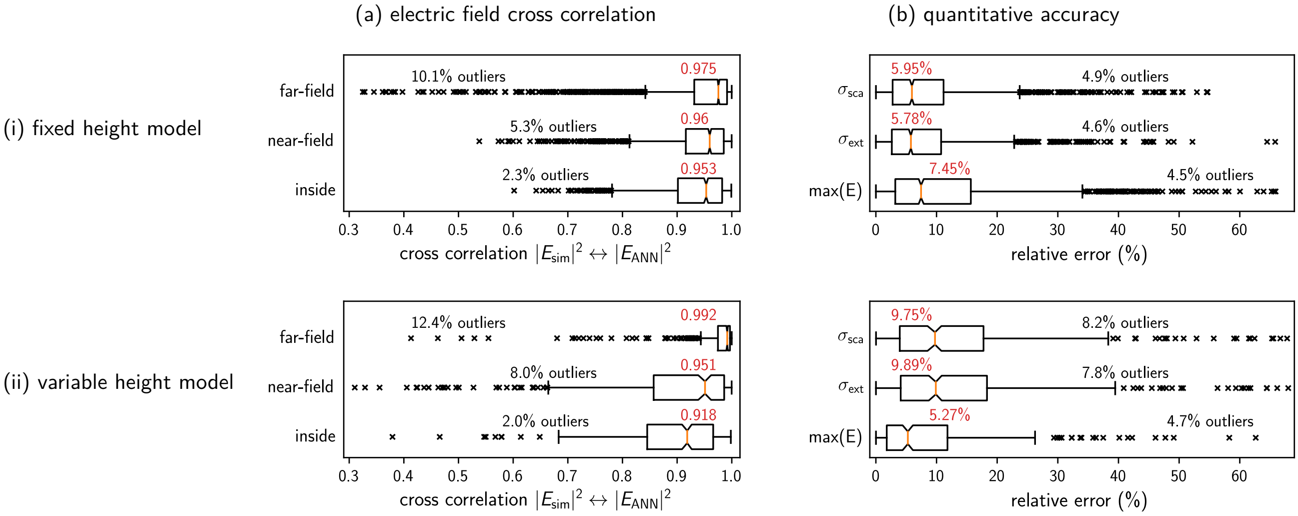


FIG. S9. Statistics on comparison between the ANN predictions and GDM simulations for the fixed (i) and variable height (ii) silicon models. The fixed height model data is identical to what is shown in the main text figure 5. (a) Qualitative comparison of field intensity distribution, in the far-field (comparing the back focal plane mappings), in the near-field in a plane 45 nm and inside the structure. (b) Relative error of the ANN (in %) for the scattering and extinction cross sections, and for the maximum value of near-field intensity.

To assess the accuracy in case of non-constant thickness nanostructures, we generated a further data-set of 20000 silicon cuboid structures with variable height. The geometric model is identical to the silicon model used in the main text (see figure S2a), with the difference that each silicon block has a random height between 60 nm and 200 nm. We evaluate this network on 500 additional random structures. These statistics are compared in figure S9 to the fixed thickness silicon model of the main text. This comparison shows, that the ANN trained on variable height is performing similarly to the ANN trained on fixed height data, with a tendency of a slightly decreased prediction accuracy. We note that the decrease in accuracy might also be due to the $\approx 30\,\%$ lower number of training data. However, an exhaustive analysis of the precise impact of different geometric models on the generalized predictor performance is out of the scope of the current work.

## IX. TRAINING CONVERGENCE

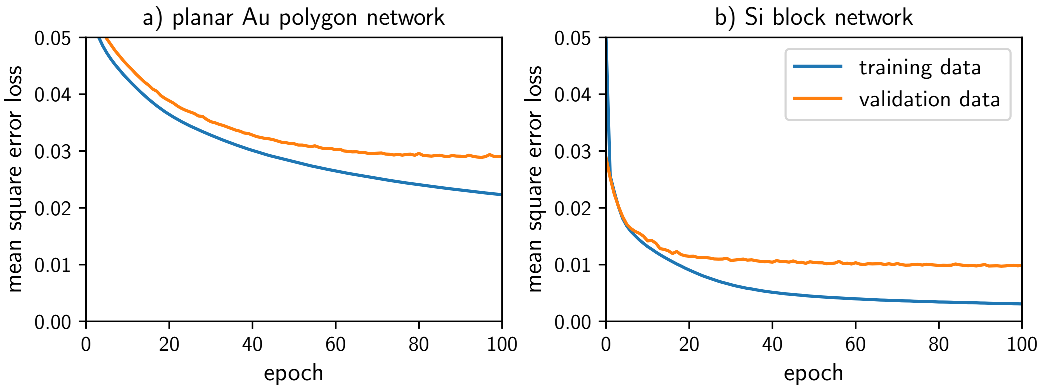


FIG. S10. Training convergence of (a) the gold-polygon network and (b) the silicon block network.

Figure S10 shows the mean square error loss of the neural network for (a) gold and (b) silicon nanostructure field prediction. Loss on training data is shown in blue, validation loss as orange lines. After 100 epochs of training no further improvement on neither set was observed for the validation data.

[S1] C. Girard, Reports on Progress in Physics **68**, 1883 (2005).
[S2] P. R. Wiecha, Computer Physics Communications **233**, 167 (2018).
[S3] C. Girard, A. Dereux, O. J. F. Martin, and M. Devel, Physical Review B **52**, 2889 (1995).
[S4] C. Girard, E. Dujardin, G. Baffou, and R. Quidant, New Journal of Physics **10**, 105016 (2008).
[S5] P. B. Johnson and R. W. Christy, Physical Review B **6**, 4370 (1972).
[S6] D. F. Edwards, in *Handbook of Optical Constants of Solids*, edited by E. D. Palik (Academic Press, Burlington, 1997) pp. 547 – 569.
[S7] C. Szegedy, S. Ioffe, V. Vanhoucke, and A. Alemi, arXiv:1602.07261 [cs] (2016), arXiv:1602.07261 [cs].
[S8] O. Ronneberger, P. Fischer, and T. Brox, arXiv:1505.04597 [cs] (2015), arXiv:1505.04597 [cs].
[S9] K. He, X. Zhang, S. Ren, and J. Sun, arXiv:1512.03385 [cs] (2015), arXiv:1512.03385 [cs].
